# Supplementary material for: Driving and characterizing nucleation of urea and glycine polymorphs in water
Source: arXiv:2210.04822 source file (2022-12-02)
Supplement: Supplementary file 1 [file SI.pdf]

---

**Supplementary Information: Driving and  
characterizing nucleation of urea and glycine  
polymorphs in water**

---

**Zou, Beyerle, Tsai and Tiwary**

## I. INTERMOLECULAR ANGLE FORMALIZATION

Here we illustrate the reason why a switching function is used in the main text while defining intermolecular angle OPs,  $\bar{\theta}_1$  and  $\bar{\theta}_2$ , in the **Order parameters for nucleation**. The probability distributions of intermolecular angles of C-O and N-N vectors of urea are plotted with dashed lines in Fig.S1. Since these angles are related to local environment and are calculated over a large population, they can not directly serve as OPs in classifying states. Instead we consider their average values as a global representation of the simulation box. As marked by the vertical lines, one is not able to identify liquid and solid state on basis of the mean value of raw angles if directly used. Instead by the use of a switching function which we quantified in **Order parameters for nucleation** Eq. 5 in the main text we find that the resulting mean values are fairly distinct between liquid and solid phases (solid lines in Fig.S1.), thereby leading to much better demarcating OPs.

## II. CLASSIFYING UREA POLYMORPHS

Here we describe the SMAC OPs mentioned in **Urea - Comparison with previous studies** of the main text [1]. This set of OPs expressed by Eq.1 maps specific angles with kernel functions using tunable cutoffs for distance  $r_{ij}$  between the  $i$ - and  $j$ -th molecules, and the number of neighbors  $n_i$  of the  $i$ -th molecule.

$$\Delta\Gamma_i = \frac{\rho_i}{n_i} \sum_{j=1}^N f_{ij} \Theta_{ij} \quad (1)$$

where density of molecule  $i$  is defined by a switching function with tunable parameter  $b$  and cutoff  $n_{cut}$ ,

$$\rho_i = \frac{1}{1 + e^{b(n_{cut} - n_i)}} \quad (2)$$

number of neighbors  $n_i$  is the summation of individual local coordination number  $f_i$  with  $a$  tuning on the sharpness of the switching function and threshold  $r_{cut}$ ,

$$n_i = \sum_{j=1}^N f_{ij} \quad (3)$$

$$f_i = \frac{1}{1 + e^{a(r_{cut} - r_i)}} \quad (4)$$

and  $\Theta_i$  describes the global orientation of molecules within the simulation box in reference of characteristic orientation  $\theta_{ij}$ ,

$$\Theta_{ij} = \sum_{k=1}^{k_{max}} e^{-\frac{(\theta_{ij} - \theta_k)^2}{2\sigma_k^2}} \quad (5)$$

where  $\sigma_k$  tunes of widths Gaussians. Given  $\Delta\Gamma_i$  represents the crystallinity of molecule  $i$  with respect to target structure, we then compute the size of nuclei of crystalline structures (denoted as  $N_{crystal}$ ) incorporating with depth first search algorithm. As shown in Fig. S2(a), liquid and solid phases (besides amorphous structures) possess completely different angular distribution functions, which makes it reasonable of the application of SMAC OPs. All configurations for these computations are drawn from WTmetaD simulations biasing SPIB-learned RCs and each trajectory is 12 ns long with a time step of 1 ps. By using these distributions as references, the population of corresponding polymorphs can be computed in combination of SMAC OPs by proper placement of switching functions and depth first search method as suggested in Ref.2. Fig. S2(b) shows estimates of size of polymorphic urea sampled, and the system is labeled by a specific phase when the cluster size,  $N$ , is greater than 50 (red dashed line).

## III. COMPETING UREA NUCLEATION PATHWAYS SEEN WITH STRONGER METADYNAMICS BIAS

Multiple nucleation pathways in aqueous solution of urea are noticed when stronger Gaussian height ( $4 k_B T$ ) is applied in WTmetaD and here we present them in details. In Fig.S3 we have plotted  $\bar{\theta}_1$  and  $\bar{\theta}_2$  with respect to

simulation time, as these serve as indicators of potential crystal formation in urea. Distinct changes in the values of these OPs can be observed after around 50 ns. In particular, two pathways are identified and boxed with dashed lines. The first pathway (top panel) corresponds to a typical two-step nucleation mechanism where amorphous cluster forms initially followed by crystallization to a ordered crystalline structure B-urea. The second pathway associates to a more complex transition consisting of crystallization and solid-solid transition. It is observed that crystal structure A-urea forms first from liquid state of urea and it undergoes a solid-solid transition to crystal form I as nucleus grows and is in agreement as reported in Ref. 3.

#### IV. CLASSIFYING GLYCINE POLYMORPHS

Since there exists no universally accepted method of classifying glycine crystal structures from all-atom simulations, each frame of the ten replicate simulations were clustered by manual inspection of the MD trajectories. The main criterion for classification is the axial representation put forth in Ref. 4 and explained thoroughly in the main text. To our knowledge, only one study has successfully assigned glycine structures to polymorphs from simulation [5]; however, Ref. 5 utilizes a coarse-grained model, not an atomistic one. While we could have coarse-grained our analysis, the template matching scheme proposed in Ref. 5 is rather involved and may not have been robust given the small size of the glycine clusters found in our simulations and the size of the template required for the method put forth in Ref. 5. Given that this study is the first (to our knowledge) to propose and utilized enhanced sampling coordinates specifically designed for crystallization of glycine, we feel that the rather ‘low tech’ approach of manual classification is acceptable and that development of more robust and powerful techniques and algorithms for the automatic classification of glycine crystal forms will be the subject of future research. An alternative technique for classifying the glycine polymorphs, which is also, admittedly rather crude, is selecting, manually, a representative structure for each polymorph observed in the simulation (as given, e.g., in Figure 5 of the main text) and performing a Voronoi tessellation of the  $(\bar{\theta}_1, \bar{\theta}_2)$  surface with the locations of the representative polymorph structures as the center of the Voronoi cells. The metadynamics weight of each structure inside a polymorph’s cell is assigned to that polymorph’s reweighted probability for the relative free-energy calculation, such as that given in Figure 7 of the main text. The relative free-energy of each polymorph found when using this Voronoi tessellation technique is given in Figure S4.

Figure S4 shows that the Voronoi tessellation method gives the  $\alpha$  and  $\beta$  polymorphs significantly lower free-energy compared to the manual clustering method, even disturbing the relative ranking relative (form  $\beta > \text{form } \gamma > \text{form } \alpha$ ) to the manual classification approach. The rationale for this is that the Voronoi tessellation method allocates

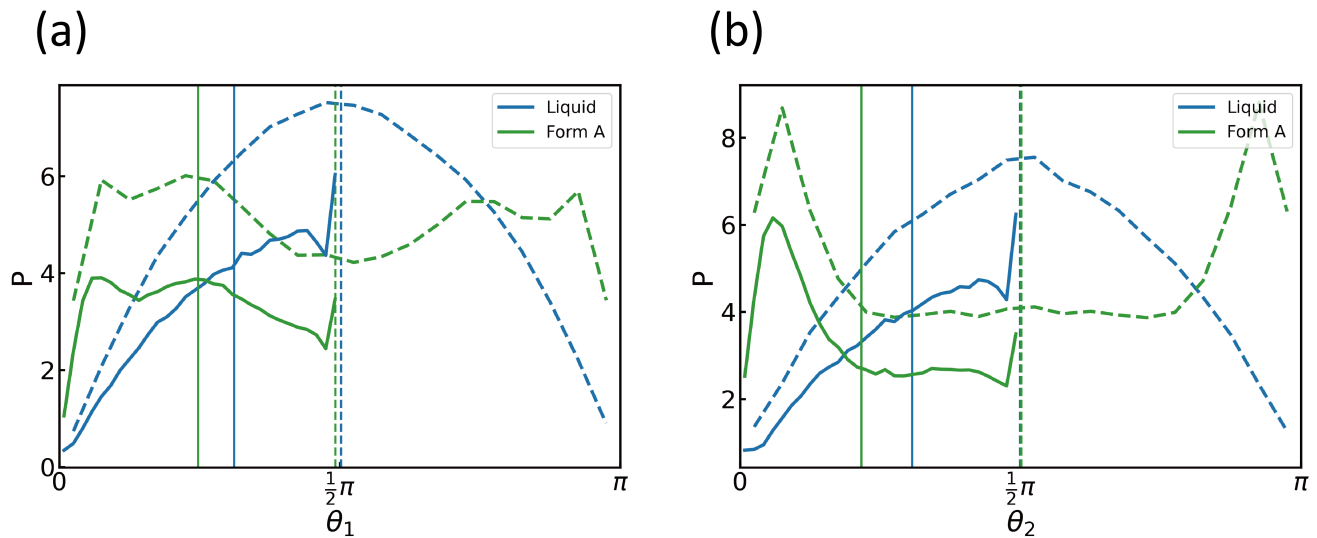

**FIG. S1:** Probability distribution of intermolecular angle,  $\theta_1$  and  $\theta_2$  for liquid (in blue) and solid (in green) urea. Geometric information is obtained from snapshots of WTmetaD simulations basing SPIB-learned RCs discussed in the main text. Dashed lines are the distributions the original OP values, and solid lines correspond to the distribution of angle values after using switching function (see main text for details). Vertical lines indicate the mean values of corresponding distributions.

TABLE S1: Classification of glycine into  $\alpha$ ,  $\beta$ , or  $\gamma$  polymorph by simulation time (in nanoseconds for all) and simulation number. All other frames in the simulation sampled the liquid state, unless otherwise noted. A horizontal line in a cell indicates the given polymorph is not sampled during the simulation.

| Sim. | $\alpha$     | $\beta$     | $\gamma$                               |
|------|--------------|-------------|----------------------------------------|
| 1    | —            | 37.0 - 49.0 | 17.75 - 22.4                           |
| 2    | 43.25 - 45.5 | —           | 16.75 - 22.85; 45.51 - 58.0            |
| 3    | —            | —           | 15.0 - 20.0; 50.0 - 78.5               |
| 4    | 75.0 - 85.0  | —           | 16.0 - 22.5; 85.0 - 88.56              |
| 5    | 52.0 - 65.0  | 12.5 - 15.0 | 15.0 - 20.0; 65.0 - 74.0               |
| 6    | 57.5 - 70.0  | 37.0 - 41.5 | 15.0 - 20.5                            |
| 7    | —            | 37.0 - 44.5 | 16.75 - 20.0; 61.0 - 71.0              |
| 8    | 39.5 - 52.0  | —           | 15.0 - 19.75; 34.0 - 39.5; 53.5 - 56.5 |
| 9    | 40.0 - 50.0  | —           | 15.15-21.0; 50.0 - 57.0                |
| 10   | 55.0 - 56.5  | —           | 15.25 - 21.75; 71.75 - 80.83           |

significantly larger neighborhoods to the polymorphs and shrinks the neighborhood allocated to the liquid state. Thus, as the area in  $(\theta_1, \theta_2)$  space ‘stolen’ by the polymorphs, compared to the manual clustering method, has higher metadynamics weight, the relative free energies for the  $\alpha$  and  $\beta$  polymorphs are lowered by an order of magnitude. We believe the manual clustering is more rigorous, which is why it is reported as the ‘ground truth’ in the main text. The simplistic Voronoi tessellation method reported in this section assigns too large of a volume in the input parameter space to the  $\alpha$  and  $\beta$  polymorphs, which are sampled much less frequently than the  $\gamma$  polymorph, thus assigning to them what we believe a too low relative free-energy.

To make the neighborhood assignments from each method clear, Figure S5 shows the neighborhoods for the liquid state and the three glycine polymorphs defined using the manual clustering technique (Figure S5(a)) and using the Voronoi tessellation procedure (Figure S5(b)). From the comparison, it is clear that, while the clustering near the representative structure are similar, the polymorph neighborhoods are much larger when using the Voronoi method. The larger neighborhood methods for the polymorphs both increase the weights assigned to each polymorph and decrease the weight assigned to the liquid state, leading to the lowering of the relative free-energies for the  $\beta$  and  $\alpha$  forms seen in Figure S4 as compared to Figure 7 in the main text.

As stated in the main text, the SMAC protocol for sorting the urea polymorphs is not used for glycine due to the similarities among the  $g(r, \theta)$  plots for the three glycine polymorphs, which are shown in Figure S6. All three polymorphs have minima in  $\theta_1$  and  $\theta_2$  centered at  $r \approx 0.5$  and  $0.8$  nm, While there are differences among the polymorphs in the depth and width of these wells, qualitatively there is little difference among the distribution functions. For this reason, the SMAC protocol for identifying polymorphs, which relies on there being large qualitative differences in the  $\theta_1$  and  $\theta_2$  values sampled by the polymorphs, is suitable for urea, where large differences in the polymorph-dependent  $g(r, \theta_i)$  are seen (Figure S2), but not for glycine. Due to this characteristic of the glycine polymorphs, the structures were instead classified manually, as previously described.

Finally, Figure S7 shows the projection of  $S(r, \theta_1)$  and  $S(r, \theta_2)$  onto  $(\bar{\theta}_1, \bar{\theta}_2)$ . A visual inspection of Figure 6(d) in the main text and Figure S7 shows that the first reaction coordinate learned from the linear SPIB used for subsequent biasing is qualitatively similar to  $S(r, \theta_1)$  without performing any calculations; this similarity is further borne out by inspection of the rescaled coefficients in Figure 6(b) of the main text. This comparison insinuates SPIB is finding a good crystallization coordinate because the liquid to solid transition is characterized by a large drop in  $S(r, \theta_1)$  and  $S(r, \theta_2)$ [6].

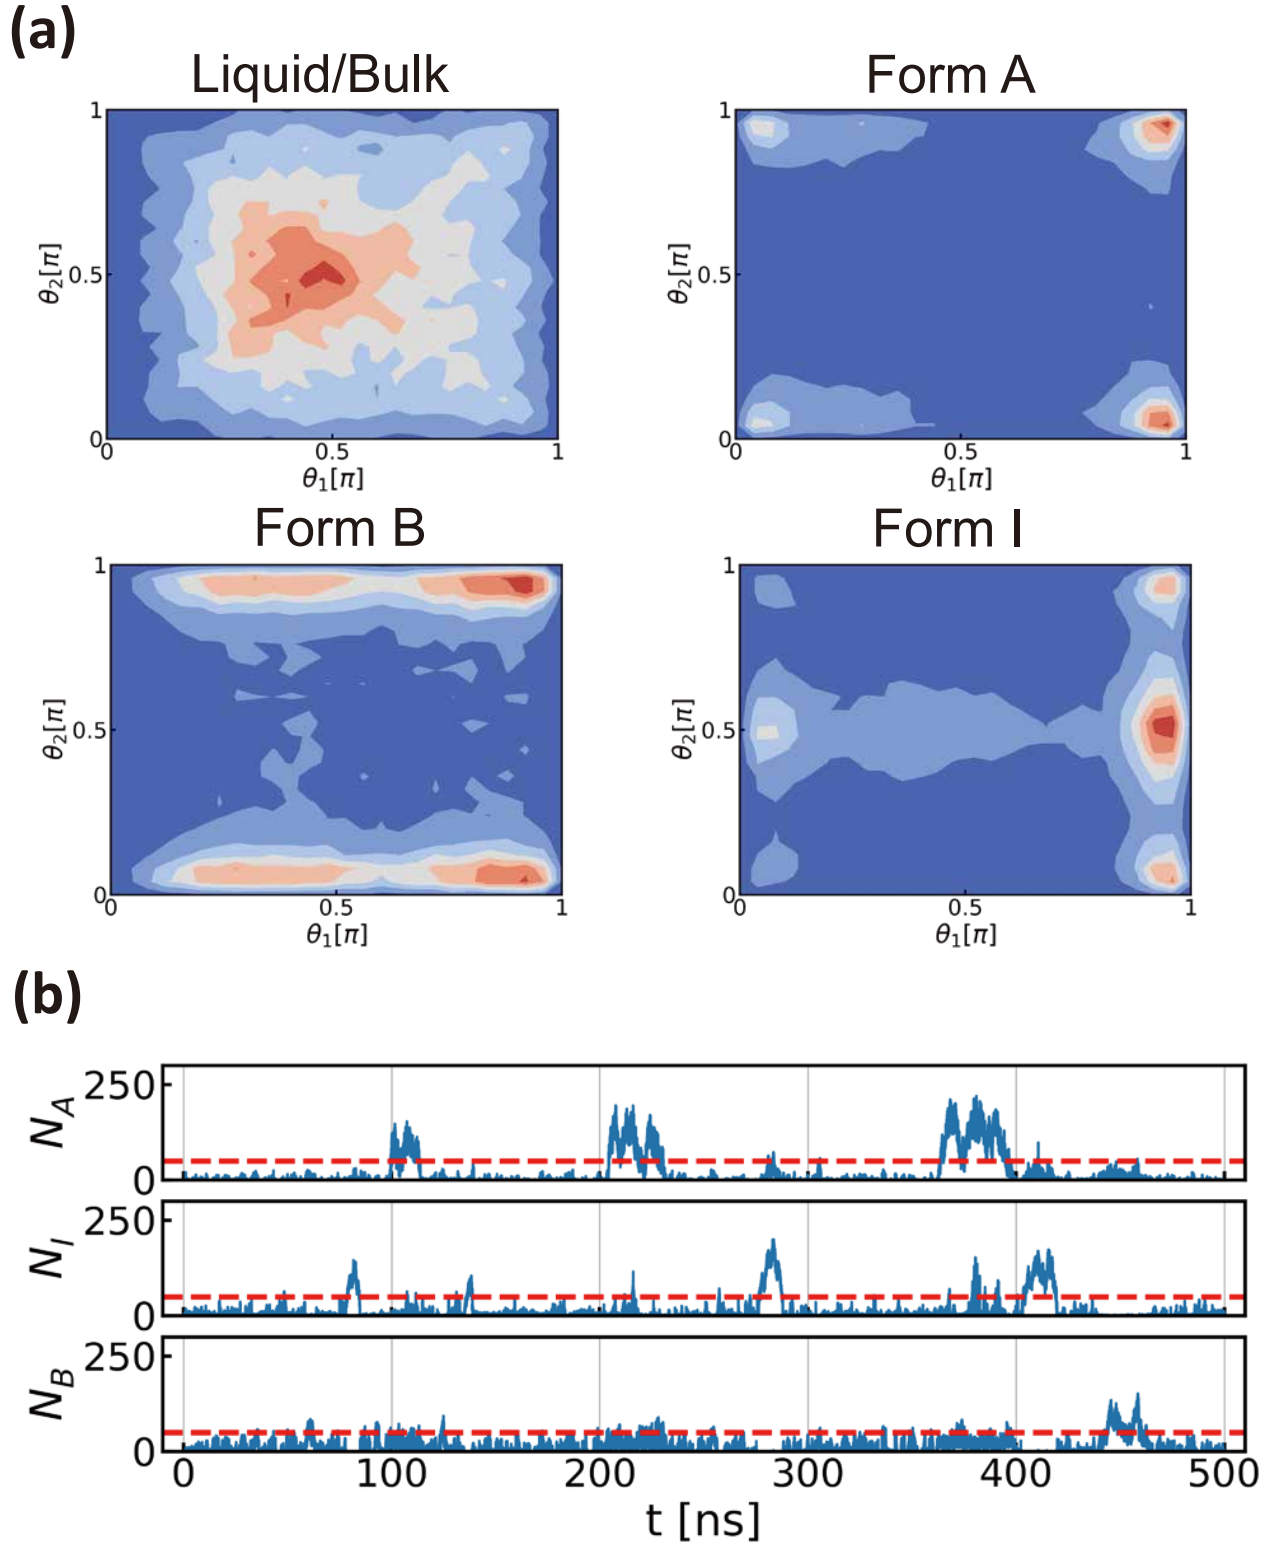

**FIG. S2:** Definitions of liquid and solid urea in angular space (panel a) and post-processed time series of crystal urea in term of cluster size (panel b). Red dashed lines are the threshold in state identification for the SMAC OPs described in **Urea - Comparison with previous studies.**. Values below this threshold (here 50) are considered as noise and classified to liquid phase.

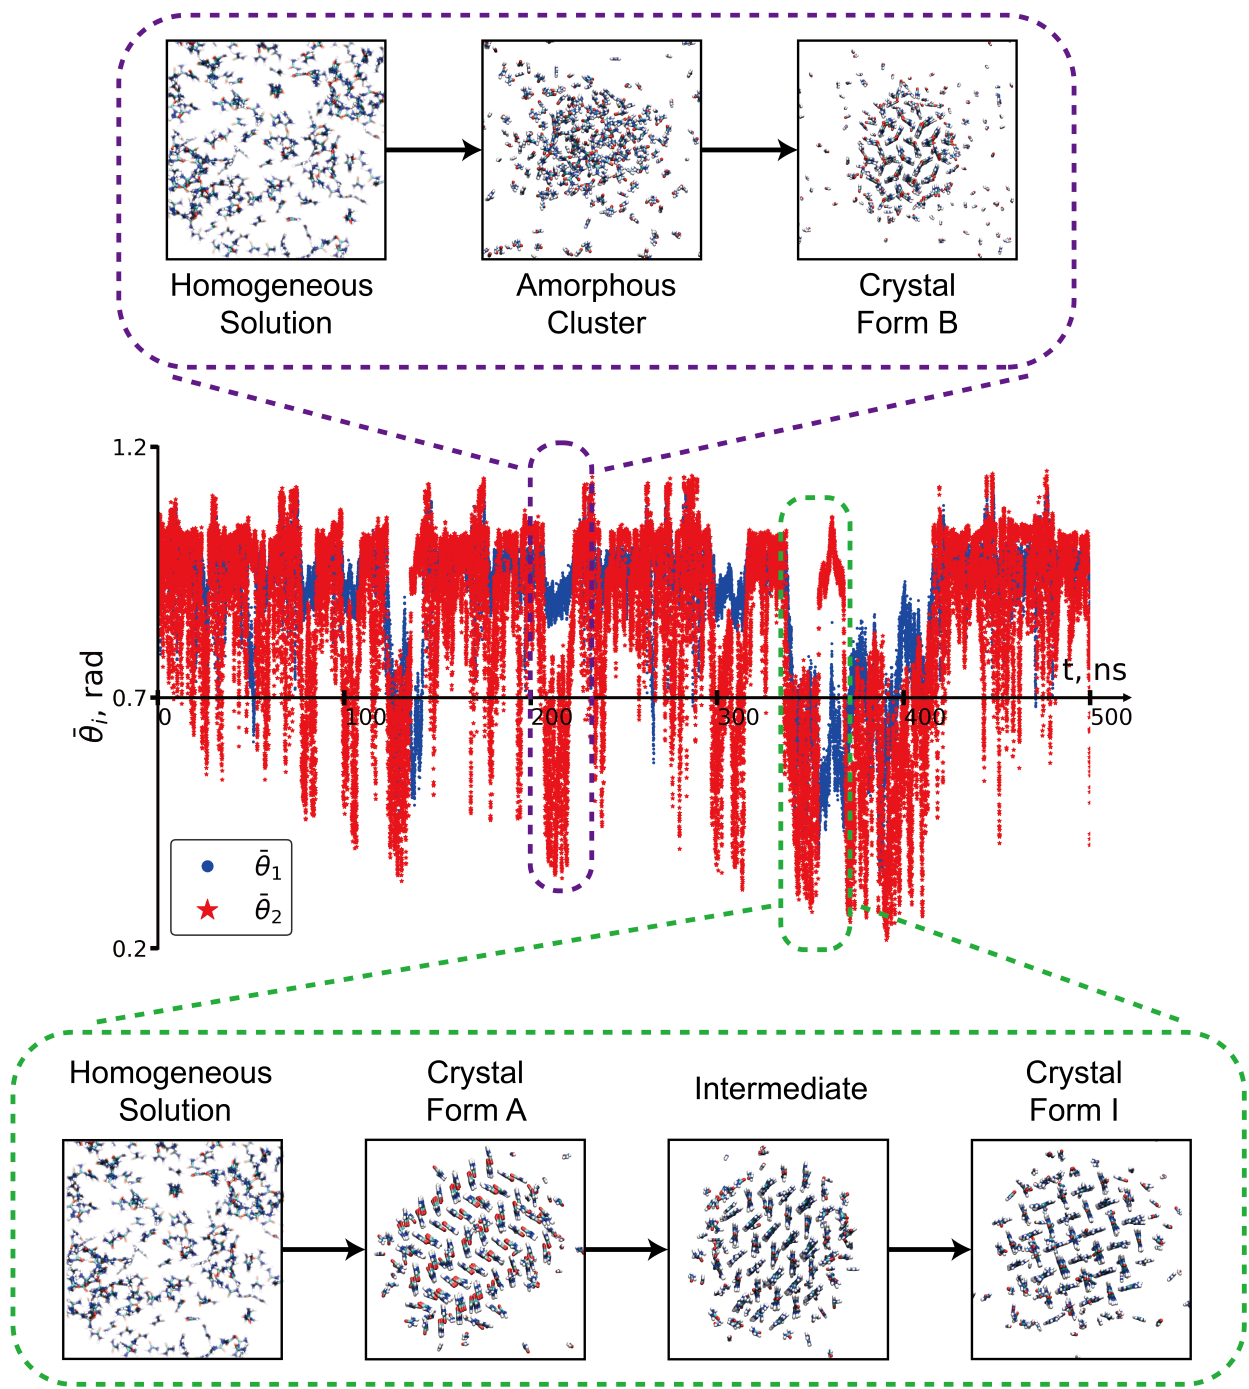

**FIG. S3:** Schematics of the two pathways of crystal nucleation of urea under strong bias. The time series of two crystalline structure identifying order parameters,  $\bar{\theta}_1$  and  $\bar{\theta}_2$ , are plotted. Two nucleation mechanisms are highlighted in dashed line and their detailed information are represented with respect to VMD snapshots.

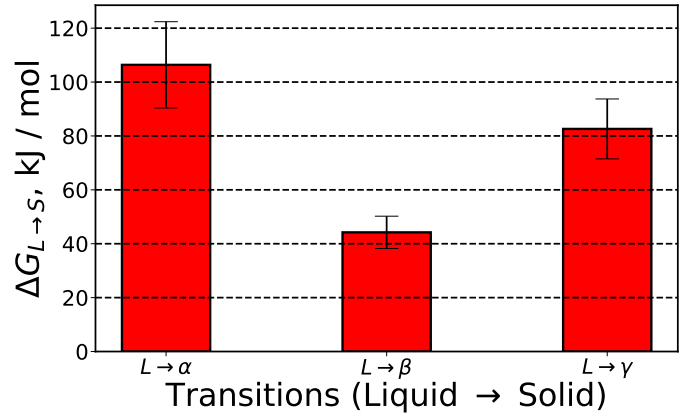

**FIG. S4:** Relative free-energy of the three predominant glycine polymorphs when using the Voronoi tessellation polymorph clustering described in Sec. IV. In contrast to Figure 7 of the main text, we find that using this protocol gives  $\beta$ -glycine as the most stable structure, followed by  $\gamma$ -glycine, then  $\alpha$ -glycine as the least stable of the three polymorphs.

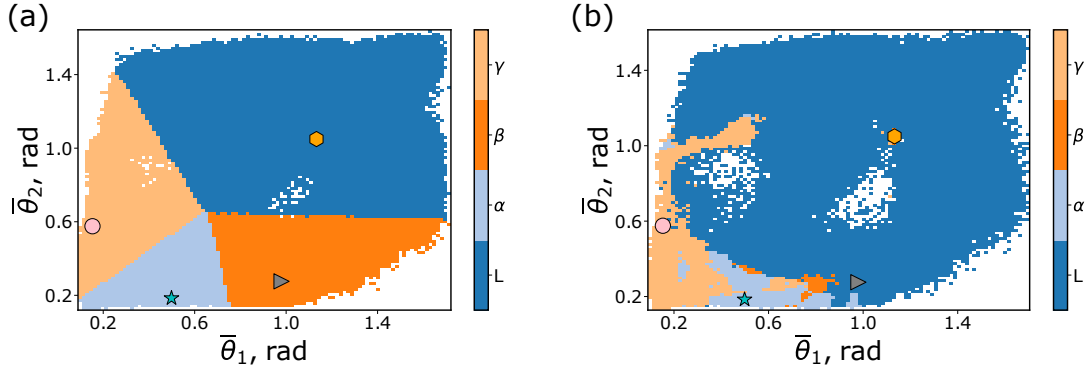

**FIG. S5:** Volume of the  $(\bar{\theta}_1, \bar{\theta}_2)$  space assigned to the liquid state (dark blue), the  $\alpha$  polymorph (light blue), the  $\beta$  polymorph (dark orange), and the  $\gamma$  polymorph (light orange) when using (a) the Voronoi tessellation assignment to a reference structure for each state and (b) the manual clustering method. The slight discrepancy between the sampling of  $(\bar{\theta}_1, \bar{\theta}_2)$  between the two figures is due to the using a trajectory sampled at 1 ps for (b) versus 0.2 ps for (a); the trajectories used for classification are otherwise identical.

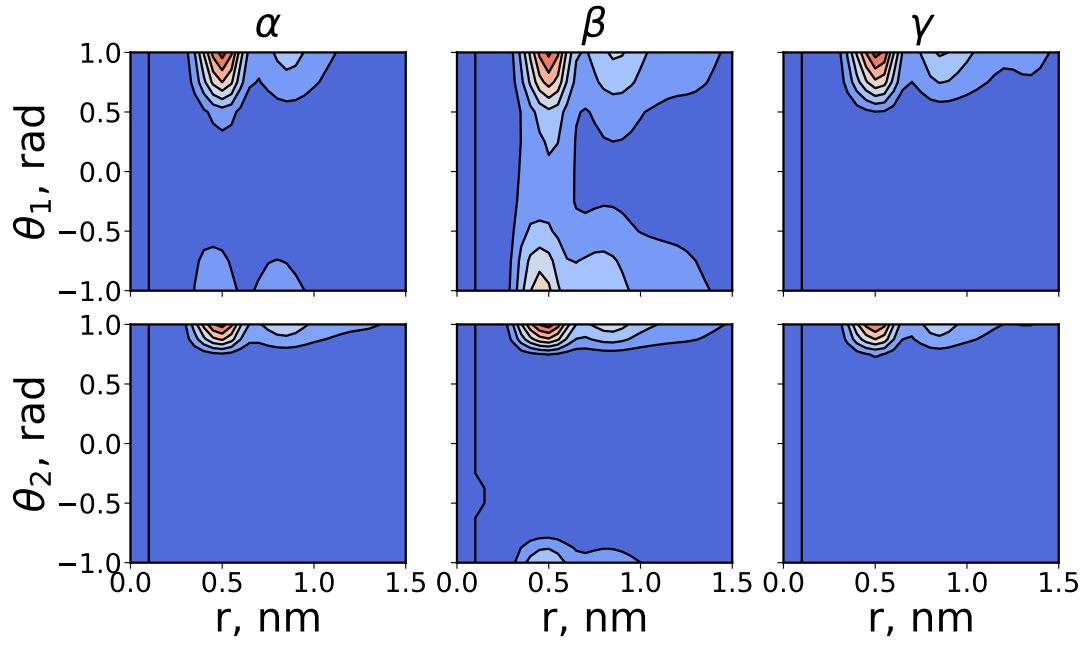

**FIG. S6:** Plots of  $g(r, \theta_1)$  (first row) and  $g(r, \theta_2)$  (second row) for the  $\alpha$  (first column),  $\beta$  (second column), and  $\gamma$  (third column) glycine polymorphs, as identified using the manual inspection protocol described in the main text.

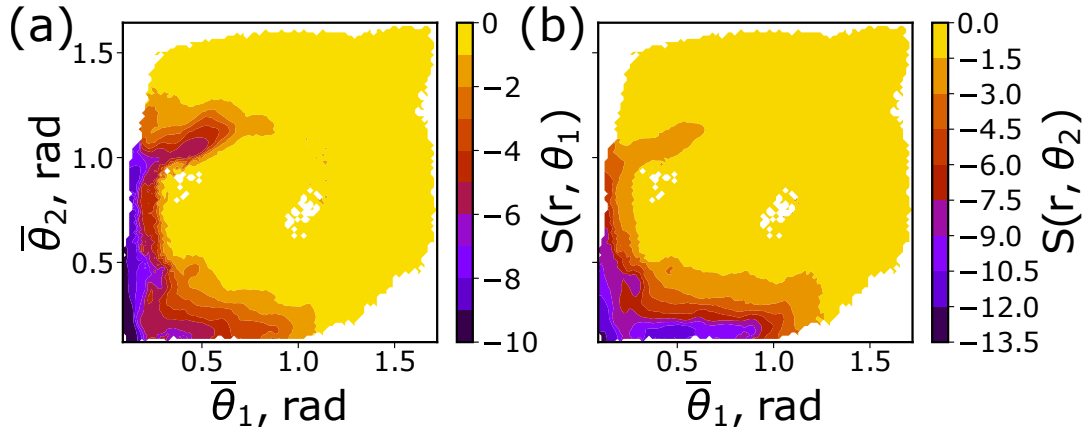

**FIG. S7:** Projection of (a)  $S(r, \theta_1)$  and (b)  $S(r, \theta_2)$  onto the space spanned by  $(\bar{\theta}_1, \bar{\theta}_2)$  for SPIB-biased simulations of glycine.

## V. RATIONALE FOR PERFORMING SPIB ON UN-REWEIGHTED TRAJECTORIES

The location of the polymorphs outside of prominent minima on the reweighted surface is partially why we do not account for the WTmetaD bias when performing the SPIB analysis [7]: while the SPIB biased simulation succeeds in sampling the polymorphs of both urea and glycine, the WTmetaD weights assigned to those states are low enough that the SPIB method does not identify them as metastable when reweighted, and, thus, fails to find a good RC (since it only ‘sees’ a single minimum) if the trajectory is reweighted during analysis.

This phenomenon is shown in Figure S8 for the glycine system in the  $(\bar{\theta}_1, \bar{\theta}_2)$  space. While the unweighted surface in Figure S8(a) shows multiple minima, including in the regions where the polymorphs exist, there is only a single minimum on the reweighted surface, centered on the liquid state, in the reweighted surface shown in Figure S8(b). While the other polymorphs reside in regions of the surface where they are clearly sampled, there is no obvious minimum capturing any of the three representative polymorph states. Since the polymorphs are located in plateaus in the surface inside of minima, they are all assigned to the same metastable state as the liquid state when SPIB is run using the reweighted trajectory. As such, for the case of nucleation presented here, reweighting in the SPIB analysis does not yield a useful set of RCs, so the unweighted trajectories are analyzed instead.

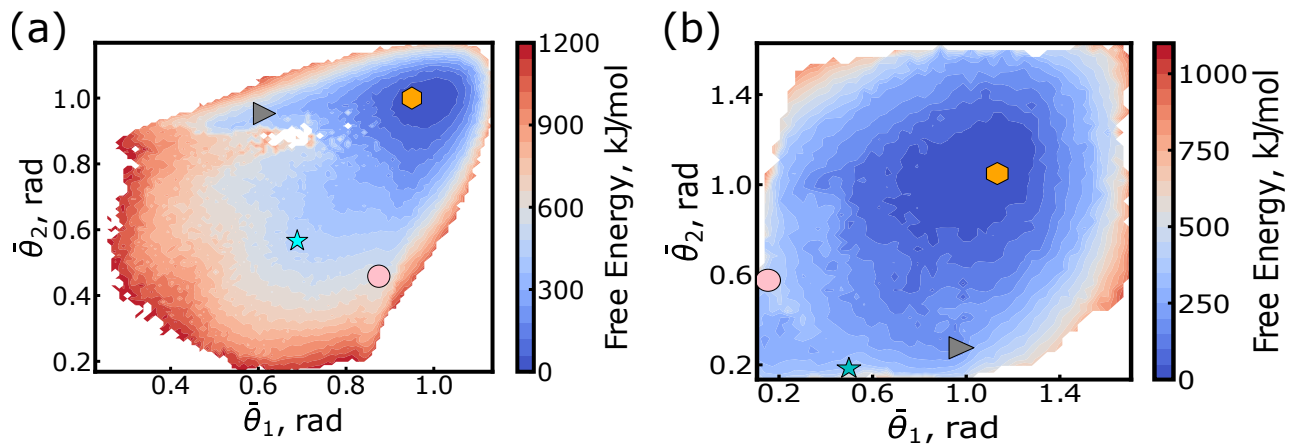

**FIG. S8:** Representative polymorph locations for urea (a) and glycine (b) (colored markers; the legend is the same as Figure 3 and S5 for urea and glycine, respectively) superimposed on the free-energy in  $(\bar{\theta}_1, \bar{\theta}_2)$  space when using the reweighted trajectory in the SPIB analysis.

## VI. COMPARISON OF SPIB-BIASED AND ENTROPY-BIASED GLYCINE SIMULATIONS

As stated in the main text, the first round of SPIB used to parameterize the SPIB coordinates for biasing the simulations of glycine analyzed in the main text is a 400-ns simulation that itself is biased along the orientational entropies,  $S(r, \theta_1)$  and  $S(r, \theta_2)$  using well-tempered metadynamics. The un-reweighted free-energy surface in  $(\bar{\theta}_1, \bar{\theta}_2)$  space and the corresponding SPIB analysis in this space are given in Figure S9.

Figure S9(a) shows the free-energy surface in the  $(\bar{\theta}_1, \bar{\theta}_2)$  space from the simulation biased along the orientational entropy OPs. The most stable minimum, as expected, is that centered at (1.0, 1.0) and corresponds to the liquid state of glycine. There is sampling of the polymorph-rich regions in the lower left-hand corner, but less so compared to the SPIB biased simulation; however, the metastable decomposition given in Figure S9 is much crisper compared to the analogous metastable decomposition for SPIB analysis with a nonlinear encoder performed on the SPIB biased simulation (data not shown). Each metastable state corresponds reasonably closely to a single crystal structure. Figures S9(c) and (d) show the projections of the two SPIB RCs onto the  $(\bar{\theta}_1, \bar{\theta}_2)$  space. The first RC,  $z_1$  is highly correlated with the  $\theta_1$  coordinate while the second RC,  $z_2$ , is highly correlated with the  $\theta_2$ . Loosely,  $z_1$  is transitions between polymorphs while  $z_2$  describes crystallization from the liquid state.

Finally, we wish to compare the exploration success of biasing with the orientational entropies compared to biasing with the linear SPIB coordinates. We perform the comparison by projecting the metadynamics weights [8]  $\exp[(V(z, t) - c(t))/k_B T]$  onto the  $(\bar{\theta}_1, \bar{\theta}_2)$  space. Figure S10(a) shows the weights from the 400-ns simulation biased along the orientational entropies and Figure S10(b) shows the weights from the SPIB-biased simulation. From the figure, it is clear that the SPIB approach assigns more weights to the volume of  $(\bar{\theta}_1, \bar{\theta}_2)$  space where the glycine polymorphs are located (colored stars in both panels of Figure S10). Because the weights in those regions are larger, the SPIB-biased simulation spends more time there and thus samples the polymorphs better than when biasing along the orientational entropy coordinates.

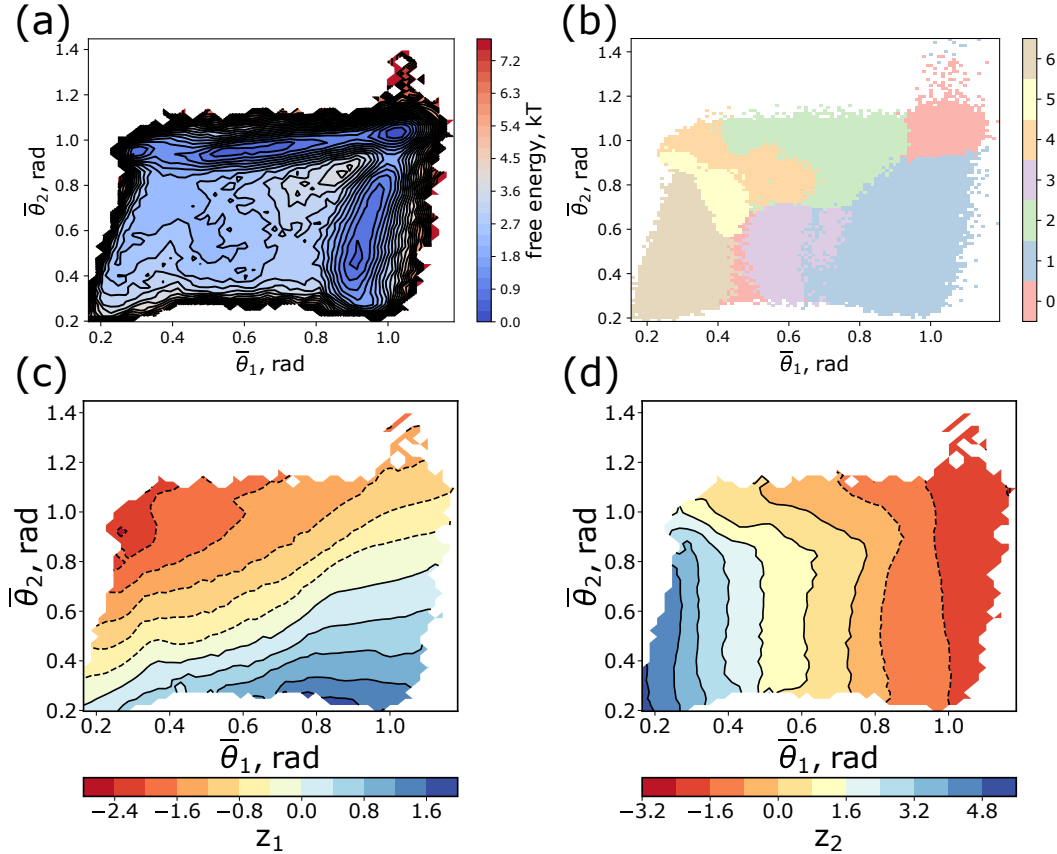

**FIG. S9:** SPIB analysis on the 400-ns aqueous glycine simulation biased along the orientational entropy OPs. (a) Un-reweighted free-energy surface. (b) Projection of the converged SPIB metastable states onto the free-energy surface. (c) Projection of  $z_1$  and (d)  $z_2$  onto the free-energy surface.

# SUPPLEMENTARY REFERENCES

- 
- [1] M. Salvalaglio, T. Vetter, F. Giberti, M. Mazzotti, and M. Parrinello, *Journal of the American Chemical Society* **134**, 17221 (2012).
  - [2] G. A. Tribello, F. Giberti, G. C. Sosso, M. Salvalaglio, and M. Parrinello, *Journal of Chemical Theory and Computation* **13**, 1317 (2017).
  - [3] M. Salvalaglio, C. Perego, F. Giberti, M. Mazzotti, and M. Parrinello, *Proceedings of the National Academy of Sciences* **112**, E6 (2015).
  - [4] Y. Iitaka, *Acta Crystallographica* **14**, 1 (1961).
  - [5] N. Duff and B. Peters, *The Journal of Chemical Physics* **135**, 134101 (2011).
  - [6] P. M. Piaggi and M. Parrinello, *Proceedings of the National Academy of Sciences* **115**, 10251 (2018).
  - [7] S. Mehdi, D. Wang, S. Pant, and P. Tiwary, *Journal of Chemical Theory and Computation* **18**, 3231 (2022).
  - [8] A. Barducci, G. Bussi, and M. Parrinello, *Physical review letters* **100**, 020603 (2008).

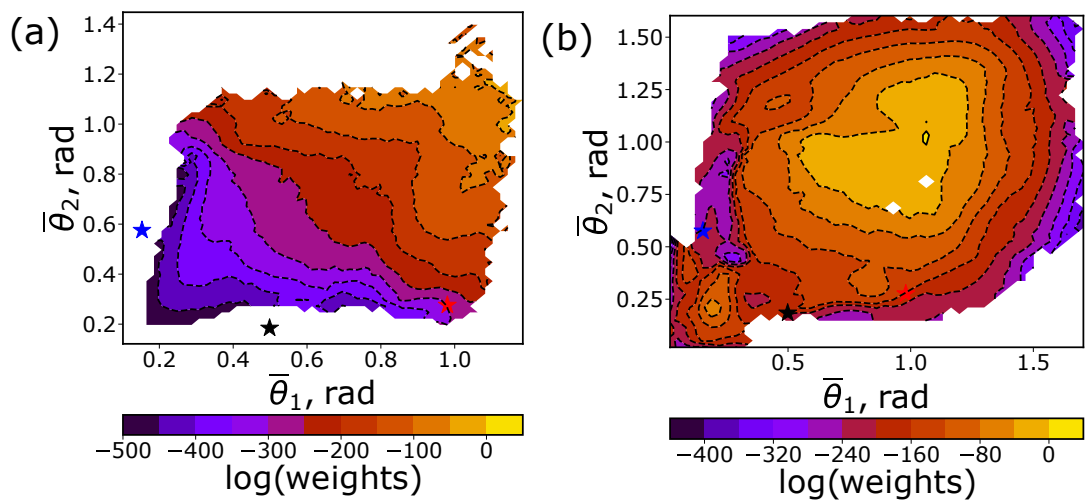

**FIG. S10:** (a) Well-tempered metadynamics weights projected onto the  $(\bar{\theta}_1, \bar{\theta}_2)$  space for the 400-ns simulation biased along the orientational entropies. (b) Same as a) but for the simulation biased along the linear, two-dimensional SPIB coordinates.
